# Supplementary material for: ThermoSight: From Appearance to Internal Thermofluid Fields via Physics-Guided Neural Reconstruction
Source: arXiv:2611.20786 source file (2026-11-16)
Supplement: Supplementary file 1 [file supp_contents.tex]

\makeatletter
\begingroup
\setcounter{tocdepth}{2}
\newcommand{\suppcontentsentry}[2]{%
  \csname l@#1\endcsname{%
    \hyperref[#2]{\numberline{\ref*{#2}.}{\let\texorpdfstring\@secondoftwo\nameref*{#2}}}%
  }{\pageref*{#2}}%
}
\suppcontentsentry{section}{sec:supp_additional_conditions}
\suppcontentsentry{section}{sec:supp_acquisition_and_implementation}
\suppcontentsentry{subsection}{sec:supp_acquisition}
\suppcontentsentry{subsection}{sec:supp_implementation}
\suppcontentsentry{subsection}{sec:supp_spectral_derivations}
\suppcontentsentry{section}{sec:supp_convergence}
\suppcontentsentry{section}{sec:supp_mismatch}
\endgroup
\makeatother
